# Supplementary material for: AIR: A Light-Weight Yet High-Performance Dataflow Engine based on Asynchronous Iterative Routing
Source: arXiv:2001.00164 source file (2020-01-03)
Supplement: Supplementary file 1 [file appendix.tex]

\begin{appendix}

\begin{algorithm}[htb]
\tiny
\vspace{1mm}
\begin{verbatim}

class Dataflow {

public:
  
  unsigned int level, worldSize, rank; // basic MPI parameters
  vector<Vertex*> vertices; // all vertices in the dataflow DAG
  
  Dataflow() {  // Initialize MPI environment 
    MPI_Init_thread(NULL, NULL, MPI_THREAD_MULTIPLE, &this->level);
    MPI_Comm_size(MPI_COMM_WORLD, &this->worldSize);
    MPI_Comm_rank(MPI_COMM_WORLD, &this->rank); }

  ~Dataflow() { // Shutdown MPI environment & clear vertices
    vertices.clear();
    MPI_Finalize(); }

  // Add a unique vertex to the DAG
  void add(Vertex* vertex) { ... } 

  // Add a unique edge among two vertices in the DAG
  void addLink(Vertex* parent, Vertex* child) { ... }

  // Main entry point to invoke stream processing
  void streamProcess() {

    pthread_t rootThreads[vertices.size()];

    // Start a new thread for each root vertex in the DAG
    unsigned int i = 0;
    for (vector<Vertex*>::iterator vertex = vertices.begin();
        vertex != vertices.end(); ++vertex) {

      if ((*vertex)->previous.empty()) { // a root vertex has no parent
        pthread_create(&rootThreads[i++], NULL, &startRootThread, (*vertex)); }
    }
    
    for (int j = 0; j < i; j++) { // wait to join root threads
      pthread_join(rootThreads[j], (void **) NULL); }
  }

private: 
  
  // Internal thread entry point per root vertex in the DAG
  static void* startRootThread(void* rootVertex) {

    rootVertex->startThreads();
    rootVertex->streamProcess(-1); // use dummy channel for root vertex
    rootVertex->joinThreads();

    pthread_exit(NULL);
}
\end{verbatim}
\vspace{1mm}
\caption{Dataflow C++ implementation of AIR}
\label{alg:dataflow}
\end{algorithm}

\begin{algorithm}[htb]
\tiny
\vspace{1mm}
\begin{verbatim}

class Vertex {

public:
  
  unsigned int vertexId, rank, worldSize; // basic vertex parameters
  
  pthread_t* listenerThreads; // listener threads for incoming messages
  pthread_t* processorThreads; // processor threads for incoming messages
  pthread_t* senderThreads; // sender threads for outgoing messages
 
  pthread_mutex_t* listenerMutexes; // listener thread mutexes
  pthread_cond_t* listenerCondVars; // listener thread conditional variables

  pthread_mutex_t* senderMutexes; // sender thread mutexes
  pthread_cond_t* senderCondVars; // sender thread conditional variables
  
  list<Message*>* inMessages; // array of incoming message queues (one per channel)
  list<Message*>* outMessages; // array of outgoing messages queues (one per channel)

  vector<Vertex*> next, previous; // links among vertices in the dataflow DAG

  // Constructor to initialize internal parameters, message buffers and threads
  Vertex(int vertexId, int rank, int worldSize) { ... }
  
  // Destructor (to be overwritten by each Vertex subclass)
  virtual ~Vertex() { ... }

  void Vertex::startThreads() {

    this->ALIVE = true;
    
    // Invoke one listener and processing thread per incoming channel
    int p = 0;
    for (vector<Vertex*>::iterator v = previous.begin(); v != previous.end(); ++v) {
      for (int i = 0; i < worldSize; i++) {

        int inChannel = p * worldSize + i;

        // Set current listener and processing threads' parameters 
        pthread_p params(...);

        // And then start the actual threads
        pthread_create(&listenerThreads[inChannel], NULL,
            &startListenerThread, (void*) &params);
        pthread_create(&processorThreads[inChannel], NULL,
            &startProcessorThread, (void*) &params); }
      p++; }

     // Invoke one sender thread outgoing channel
    int n = 0;
    for (vector<Vertex*>::iterator v = next.begin(); v != next.end(); ++v) {
      for (int i = 0; i < worldSize; i++) {

        int outChannel = n * worldSize + i;

        // Set current sender thread's parameters 
        pthread_p params(...);

        pthread_create(&senderThreads[outChannel], NULL,
            &startSenderThread, (void*) &params); }

      // Recursively invoke subsequent vertices' threads (if not yet alive)
      (*v)->startThreads();
      n++; }
  }

  void Vertex::joinThreads() {

    int p = 0;
    for (vector<Vertex*>::iterator v = previous.begin(); v != previous.end(); ++v) {
      for (int i = 0; i < worldSize; i++) {

        // Wait to join incoming channel's thread
        int inChannel = p * worldSize + i;
        pthread_join(listenerThreads[inChannel], (void **) NULL);
        pthread_join(processorThreads[inChannel], (void **) NULL); }
      p++; }

    int n = 0;
    for (vector<Vertex*>::iterator v = next.begin(); v != next.end(); ++v) {
      
      // Recursively join subsequent vertices' threads (if still alive)
      (*v)->joinThreads();

      for (int i = 0; i < worldSize; i++) {

        // Wait to join outgoing channel's thread
        int outChannel = n * worldSize + i;
        pthread_join(senderThreads[outChannel], (void **) NULL); }
      n++; }
      
      this->ALIVE = false;
}

  void* startListenerThread(void* params) {

    // Receive messages only with matching tag for channel
    unsigned int tag = params->fromVertex->vertexId;
    tag = (tag << 8) + params->toVertex->vertexId;
    tag = (tag << 8) + params->toRank;

    MPI_Status status;
    Message* inMessage;

    while (ALIVE) {
      
      inMessage = new Message();

      // Probe and receive inMessage at current channel
      MPI_Probe(params->fromRank, tag, MPI_COMM_WORLD, &status);
      MPI_Get_count(&status, MPI_CHAR, &inMessage->size);
      MPI_Recv(inMessage->buffer, inMessage->size, MPI_CHAR,
          status.MPI_SOURCE, status.MPI_TAG, MPI_COMM_WORLD, &status);

      // Enqueue message and notify processing thread (producer-consumer pattern)
      pthread_mutex_lock(&params->toVertex->listenerMutexes[channel]);
      params->toVertex->inMessages[params->channel].push_back(inMessage);
      pthread_cond_signal(&params->toVertex->listenerCondVars[params->channel]);
      pthread_mutex_unlock(&params->toVertex->listenerMutexes[params->channel]); }
  }

  void* startSenderThread(void* params) {

    // Generate unique message tag per channel
    unsigned int tag = params->fromVertex->vertexId;
    mTag = (mTag << 8) + params->toVertex->vertexId;
    mTag = (mTag << 8) + params->toRank;

    Message* outMessage;

    while (ALIVE) {

      pthread_mutex_lock(&params->fromVertex->senderMutexes[params->channel]);

      // Wait for conditional variable to be signalled (producer-consumer pattern)
      while (params->fromVertex->outMessages[params->channel].empty()) {
        pthread_cond_wait(&params->fromVertex->senderCondVars[params->channel],
            &params->fromVertex->senderMutexes[params->channel]); }
      
      // Send outMessage at current channel
      while (!params->fromVertex->outMessages[params->channel].empty()) {
      
        outMessage = params->fromVertex->outMessages[params->channel].front();
        params->fromVertex->outMessages[params->channel].pop_front();

        MPI_Send(outMessage->buffer, outMessage->size, MPI_CHAR, params->toRank,
            tag, MPI_COMM_WORLD);

        delete outMessage; }

      pthread_mutex_unlock(&fromVertex->senderMutexes[channel]); }
  }
}
\end{verbatim}
\vspace{1mm}
\caption{Vertex C++ implementation of AIR}
\label{alg:vertex}
\end{algorithm}

\begin{algorithm}[htb]
\tiny
\vspace{1mm}
\begin{verbatim}

class Map {

public: 

  Function* func;
  
  Map(Function* func, int tag, int rank, int worldSize, bool PIPELINE) :
      Vertex(tag, rank, worldSize) { ... }

  ~Map() { ... }


  void Map::streamProcess(int inChannel) {

    Message* inMessage, *outMessage;
    list<Message*>* tmpMessages = new list<Message*>();

    while (ALIVE) {

      // Synchronize on incoming message channel (producer-consumer pattern)
      pthread_mutex_lock(&listenerMutexes[inChannel]);
      while (inMessages[channel].empty()) {
        pthread_cond_wait(&listenerCondVars[inChannel],
            &listenerMutexes[inChannel]); }

      while (!inMessages[inChannel].empty()) {

        inMessage = inMessages[inChannel].front();
        inMessages[channel].pop_front();
        tmpMessages->push_back(inMessage); }

      pthread_mutex_unlock(&listenerMutexes[inChannel]);

      while (!tmpMessages->empty()) {

        inMessage = tmpMessages->front();
        tmpMessages->pop_front();

        Partition<int> partition;
        Serialization.deserialize(inMessage, &partition); // deserialization of incoming message
        
        // Apply actual map function to each deserialized element 
        for (int j = 0; j < partition.size(); j++) {
          partition.set(func->calculate(partition.get(j)), j); }

        // Reroute results into outgoing message channels
        int n = 0;
        for (vector<Vertex*>::iterator v = next.begin(); v != next.end(); ++v) {

          outMessage = new Message();
          Serialization.serialize(&partition, outMessage); // serialize results into outgoing message

          int outChannel = n * worldSize + rank; // determine channel for outgoing message

          if (PIPELINE) {

            // Pipeline mode: immediately copy message into next operator's incoming message queue
            pthread_mutex_lock(&(*v)->listenerMutexes[outChannel]);
            (*v)->inMessages[outChannel].push_back(outMessage);
            
            pthread_cond_signal(&(*v)->listenerCondVars[outChannel]);
            pthread_mutex_unlock(&(*v)->listenerMutexes[outChannel]);

          } else {
          
            // MPI mode: synchronize on outgoing message channel & send message
            pthread_mutex_lock(&senderMutexes[outChannel]);
            outMessages[outChannel].push_back(outMessage);
            
            pthread_cond_signal(&senderCondVars[outChannel]);
            pthread_mutex_unlock(&senderMutexes[outChannel]); }

          n++; }

        delete inMessage; // delete incoming message and free memory
        c++; }

      tmpMessages->clear(); }

    delete tmpMessages; // delete temp message buffer
}
\end{verbatim}
\vspace{1mm}
\caption{Map C++ implementation of AIR}
\label{alg:vertex}
\end{algorithm}

Note that type casting needed for the {\tt void*} pointers is omitted from the above code snippets. Destructors are also omitted.

\end{appendix}
